# Supplementary material for: Anisotropic hybridization in CeRhSn
Source: arXiv:2406.01516 source file (2024-06-03)

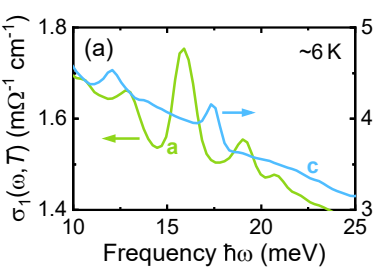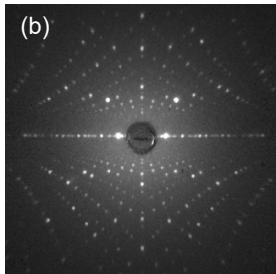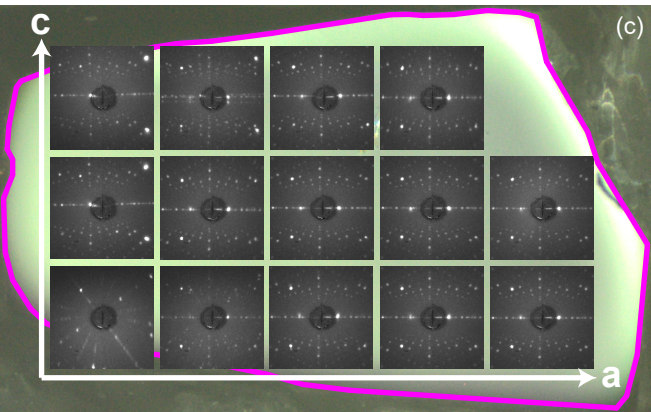

Supplement: Supplementary file 1 [file SupplementalFigure1.pdf]
